# Supplementary material for: Efficient delay-tolerant particle filtering
Source: arXiv:1009.4409 source file (2010-09-22)
Supplement: Supplementary file 1 [file appendix.tex]

\section{RTS smoother} \label{app:RTS_smoother}

In this algorithm we use the estimates of mean and covariance saved
at every previous step of the algorithm. We start with the current
distribution at time $t$, $p(x_t|y_{1:t}) \approx \mathcal{N}(x_t,
\mu_t, \bP_t)$ and propagate it using the RTS recursion as follows:
\begin{align}
\bP_{k-1|k} &= \bF_{k-1} \bP_{k-1} \bF_{k-1}^T + \bR_{k-1} \\
\bK_{k-1} &= \bP_{k-1} \bF_{k-1}^T \bP_{k-1|k}^{-1} \\
\bz_{k-1} &= \widetilde\mu_{k} - f_{k-1}(\mu_{k-1}) \\
\widetilde\mu_{k-1} &= \mu_{k-1} + \bK_{k-1} \bz_{k-1} \\
\widetilde \bP_{k-1} &= \bP_{k-1} + \bK_{k-1} (\widetilde \bP_{k} -
\bP_{k-1|k}) \bK_{k-1}^T
\end{align}
Here $f_{k-1}$ is the state transition function, $\bF_k =
\frac{\partial} {\partial x} \mathit{f}_{k}(x)|x= \mu_k$; $(\mu_k,
\bP_k)_{1\leq k\leq t}$ is the sequence of saved means and
covariances; $(\widetilde\mu_{k-1}, \widetilde \bP_{k-1})$ are the
smoothed state estimate and its covariance. After running this
recursion, initialized with $(\widetilde\mu_{t}, \widetilde \bP_{t})
= (\mu_{t}, \bP_{t})$, for $k = t, t-1, \tau+1$ we obtain the
smoothed distribution at time $\tau$, $p(x_\tau|y_{1:t}) \approx
\mathcal{N}(x_\tau, \widetilde\mu_{\tau}, \widetilde \bP_{\tau})$.
